# Supplementary material for: Low-bit Quantization for Deep Graph Neural Networks with Smoothness-aware Message Propagation
Source: arXiv:2308.14949 source file (2023-08-29)
Supplement: Supplementary file 1 [file ADMP_example.tex]

\begin{figure}[htb] 

\subfigure[no AdMP]{
\includegraphics[height=0.95in,width=2.6in]{plots/admp_method_flow_basic.jpg}\label{no_admp_example}}
\hspace{4mm}
\subfigure[AdMP with $\delta_{0}$ = 0.5]{
\includegraphics[height=0.95in,width=2.4in]{plots/admp_method_flow_ours.jpg}\label{admp_example}}
\vspace{-2mm}
\centering\caption{Illustrative Example for AdMP }
\label{admp_example_illustrative}
\end{figure}

Figure \ref{admp_example_illustrative} presents an intuitive example to show how AdMP is designed to smooth the changes in the relations between connected nodes at layer-wise message propagation. Specifically, the values over the edges represent the difference between connected nodes, e.g., for $v_1$ and $v_2$, $(\frac{\mathbf{h}_{1}}{\sqrt{d_{1}}} -\frac{\mathbf{h}_{2}}{\sqrt{d_{2}}})$ = -0.6. Figure \ref{no_admp_example} show a case that the correlations between connected nodes get sharp changes. In AdMP, with the constraints of $\delta_{0}$ = 0.5, the changes of the relations between $v_1$ and $v_2$ get smooth from layer $l$ to $l+1$, which can be friendly to get stable representation and avoid missing optimal point.
