# Supplementary material for: Low-bit Quantization for Deep Graph Neural Networks with Smoothness-aware Message Propagation
Source: arXiv:2308.14949 source file (2023-08-29)
Supplement: Supplementary file 2 [file quantization_error_analysis.tex]

If the de-quantized value is represented as $\hat{U}=(U_q- z)s$, the mean squared error (MSE) or total average distortion between $U$ and $Q(U)$ 
% \TG{check this, what you have in the equation is $U$ and $D(U_q)$} 
is given by
%Therefore, the mean sq\hat{\alpha}uared error(also called total average distortion) between $U$ and $Q(U)$ can be written as follows:
\begin{equation}
% \centering
\small
\begin{aligned}
E[(U - \hat{U})^{2}] =% \int_{-\infty}^{\infty}f(u)(u-\hat{u})^2dx \\&
\underbrace{\int_{-\infty}^{\alpha}f_U(u)(u-\hat{\alpha})^2 du}_\text{overload} + %\\
%&
\underbrace{\sum_{i=0}^{2^b-1}\int_{\alpha+i\Delta}^{\alpha+(i+1)\Delta}f_U(u)(u-\hat{u})^2du}_\text{granular} %\\&
+ \underbrace{\int_{\beta}^{\infty}f_U(u)(u-\hat{\beta})^2du}_\text{overload}
\end{aligned}
\label{eq:quantized_MSE}
\end{equation}
% \begin{equation}
% \begin{aligned}
% \int_{\alpha}^{\beta}f(u)(u-\hat{u})^2dx  \approx % \int_{-\infty}^{\infty}f(u)(u-\hat{u})^2dx \\&
%   \int_{\alpha}^{\beta}f(u)(u-\hat{u})^2dx 
% \end{aligned}
% \label{eq:quantized_MSE}
% \end{equation}
% \TG{what are $\hat{\alpha}$ and $\hat{\beta}$? don't think you have mentioned before.}

The MSE consists of three terms combining \emph{overload distortion}, $E_{ol}$, caused by the clipping operation for values of $u$ beyond $[\alpha, \beta]$, and \emph{granular distortion}, $E_{gran}$ the quantization error introduced by the quantization step $\Delta$. 
For any $U=u \in [\alpha, \beta]$, its granular distortion is in $[-\frac{\Delta}{2},\frac{\Delta}{2}]$ depending on $f_U(u)$. %the probability density distribution of the input. 
%The size of $\Delta$ is determined by $[\alpha, \beta]$ and the quantization levels 2$^b$, 
%a smaller quantization level will enlarge $\Delta$ and further increase the quantization error. 
% The larger the value of $\Delta$, the larger is the quantization error. 
Therefore, $E_{gran}$ can be reduced by setting the proper 
% \TG{optimal?}
$\Delta$ according to the distribution of $U$.

% For simplicity, given a value  $u \in [\alpha, \beta]$, its quantization error can be written as:
% \begin{equation}
% f_{e}(u) = \|u - \hat{u}\|^{2} = \|s(\frac{u}{s} - \lfloor\frac{u}{s}\rceil)\|^{2}
% \label{eq:quantization_error_two_sources}
% \end{equation}
% The quantization error comes from two sources, i.e., $s$ and $\frac{u}{s} - \lfloor\frac{u}{s}\rceil$, which are the quantization level and the distortion caused by rounding operation, respectively.
